# Supplementary material for: Motion Informed Needle Segmentation in Ultrasound Images
Source: arXiv:2312.01239 source file (2024-05-04)
Supplement: Supplementary file 1 [file appendix.tex]

%  \begin{figure}[h!]
%     \centering
%     \includegraphics[width=0.8\linewidth, height=4cm]{figures/conv_kalman_sequence.png}
%     \caption{Qualitative performance of the proposed method on test data. (a) a sequence of ultrasound images with the needle occluded in the middle due to nerve. (b) needle mask prediction overlayed in red from the proposed method. The prediction improves with time showing the efficacy of the proposed method.}
%     \label{fig:conv_kalman_sequence}
% \end{figure}

% \begin{table}
% \caption{Table captions should be placed above the
% tables.}\label{tab1}
% \begin{tabular}{|l|l|l|}
% \hline
% Heading level &  Example & Font size and style\\
% \hline
% Title (centered) &  {\Large\bfseries Lecture Notes} & 14 point, bold\\
% 1st-level heading &  {\large\bfseries 1 Introduction} & 12 point, bold\\
% 2nd-level heading & {\bfseries 2.1 Printing Area} & 10 point, bold\\
% 3rd-level heading & {\bfseries Run-in Heading in Bold.} Text follows & 10 point, bold\\
% 4th-level heading & {\itshape Lowest Level Heading.} Text follows & 10 point, italic\\
% \hline
% \end{tabular}
% \end{table}


% \begin{table}[h]
%     \centering
%     \begin{tabular}{c| c c c}
%     Method & $N=7$ & $N=20$ & $N=35$
%     \\
%     \hline
%     \\
%     DSC  & 0.577 $\pm$ 0.006 & 0.473 $\pm$ 0.010 & 0.373 $\pm$ 0.010
%     \\
%     Precision & 0.603 $\pm$ 0.006 & 0.647 $\pm$ 0.005 & 0.679 $\pm$ 0.002
%     \\
%     Recall & 0.627 $\pm$ 0.012 &  0.442 $\pm$ 0.100 & 0.373 $\pm$ 0.020
%     \end{tabular}
%     \caption{Our method's performance with different sequence lengths ($N$)}
%     \label{table:convkalman_comp}
% \end{table}

% Within the ConvKalman block, we vary the sequence length ($N$) of images as mentioned in the Section \ref{sec:training} during training. We compare the results of our network with sequence lengths of 7, 20, and 35. Since the sequence length governs the re-initialization of the ConvKalman block, we observe that having a higher sequence length results in saturation of the ConvLSTM model.Therefore, from Table \ref{table:convkalman_comp} it can be seen that shorter length sequence, $N=$7 performs better than others.


% Lastly, as mentioned earlier, we also try using optical flow as an additional input apart from the image frame.  We use U-Net with a small modification based on \cite{simonyan2014two} where the optical flow and the image are first propagated through CNNs and then the generated feature maps are added and propagated through the U-Net. This method performs poorly with a Dice Score of 0.09, which we believe was due to poor optical flow values as the ultrasound images have high background movement and noise. 

% We also try curriculum based approach where we first train the UNet, then we train the motion model along with the Unet decoder and then we fine-tune the entire network. 
% Lastly, as mentioend earlier, we also use optical flow as an input similar to the network in (cite two-stream) with the change that after passing the image and optical flow through the CNN, we add both feature maps and then pass it as an input to the Unet, the results of this as shown below. 
% We further show that the proposed network doesn't predict needle when no needle is present in the image, while Vanilla UNet fails to do so and predicts non-existing needles (add qualitative:images results for this)


% \begin{table}[h]
%     \centering
%     \begin{tabular}{c| c c c}
%     Encoder & Vanilla & ConvLSTM & ConvKalman Block
%     \\
%     \hline
%     \\
%     ResNet-50  &  $\pm$  &  $\pm$  &  $\pm$ 
%     \\
%     TransUNet encoder &  $\pm$  &  $\pm$  & $\pm$ 
%     % \\
%     % Recall & 0.627 $\pm$ 0.012 &  0.442 $\pm$ 0.100 & 0.373 $\pm$ 0.020
%     \end{tabular}
%     \caption{to be written}
%     \label{table:convkalman_comp}
% \end{table}


% \begin{figure}
% \centering
% % \includegraphics[width=18cm]{figures/SequenceLen_NetworkArchitecture.jpg}
% \includegraphics[width=0.9\textwidth]{figures/conv_kalman_net_diagram.png}
% \caption{An image is propagated through the encoder to get image features. The lowest level feature is propagated through ConvKalman block which has an estimate of the feature based on previous image. The feature is propagated  through the Prediction Step and Update Step to get the filtered feature. Finally, the filtered feature is propagated through the decoder to generate segmentation mask.}
% \label{fig:ConvKalman_Unet}
% \end{figure}
